# Supplementary material for: Optimal Pricing Schemes in the Presence of Social Learning and Costly Reporting
Source: arXiv:2211.07362 source file (2023-12-09)
Supplement: Supplementary file 1 [file Appendix_AB_discrete.tex]

\section{Appendix A: Finite Case}
\label{Section_App_A}
 
\setcounter{figure}{0}  
\subsection{Proof of Full Coverage:  Lemma \ref{FC_lemma_finite} and Proposition \ref{FC_proposition_finite} }
\subsubsection{Proof of Lemma \ref{FC_lemma_finite}}
\begin{proof}
    If the platform uses full coverage strategy the goal is:
\[
\begin{split}
\max\limits_{b} \mathbb E R_1(1+r+..+r^{t_0-1})+\mathbb E \max\{R_1,R_2\}(r^{t_0}+..+r^{T-1})-\mathbb E\text{cost}\\
\Leftrightarrow \max \limits_{b} \mathbb ER_1\frac{r^{t_0}-1}{r-1}+\mathbb E\max\{R_1,R_2\}r^{t_0}\frac{r^{T-t_0}-1}{r-1}-\mathbb E \text{cost}
\end{split}
\]
where $t_0=\min \{t|H(b_t)>c_t\}$. 

Hence we know for each agent he has probability $S_i=H(b_i)$ to report his utility. We let $a_i=Pr(t_0=i)=S_i \prod\limits_{j=1}^{i-1} (1-S_j),\forall i\le T-1$ for the probability that agent $i$ reports, and let $a_{T}=Pr(t_0=T)+Pr(\text{no reports})=\prod\limits_{j=1}^{T-1} (1-S_j)$ stand for the probability that no agents before $T$ reports. Using this notation makes $\sum\limits_1^T a_i=1$. By this definition we have 
\[\begin{aligned}
	profit=\sum\limits_{i=1}^T Pr(t_0=i)[\mathbb ER_1\frac{1-r^{i}}{1-r}+\mathbb E\max\{R_1,R_2\}\frac{r^{i}-r^T}{1-r}-b_{i}r^{i-1} ]+Pr(\text{no reports}) \mathbb ER_1\frac{1-r^T}{1-r}\\
	=\sum\limits_{i=1}^{T-1} Pr(t_0=i)[\mathbb ER_1\frac{1-r^{i}}{1-r}+\mathbb E\max\{R_1,R_2\}\frac{r^{i}-r^T}{1-r}-b_{i}r^{i-1} ]+a_T \mathbb ER_1\frac{1-r^T}{1-r}-Pr (t_0=T )b_T r^{T-1}\\
	=\sum\limits_{i=1}^{T-1} a_i [\frac{\mathbb ER_1-\mathbb E\max\{R_1,R_2\} r^T}{1-r}+\frac{Mr^i}{1-r}-b_ir^{i-1} ]+a_T \mathbb ER_1\frac{1-r^T}{1-r}-Pr (t_0=T )b_T r^{T-1}\\
	=(1-a_T)\frac{\mathbb ER_1-\mathbb E\max \{R_1,R_2\}r^T}{1-r}+\sum\limits_{i=1}^{T-1} a_i r^i\frac{M-b_i(1-r)/r}{1-r}+a_T\mathbb ER_1\frac{1-r^T}{1-r}-Pr (t_0=T )b_T r^{T-1}\\
	=\sum\limits_{i=1}^{T-1} a_i r^i\frac{M-b_i(1-r)/r}{1-r}-Pr (t_0=T )b_T r^{T-1}+a_T\frac{M r^T}{1-r}+constant
\end{aligned}\]

Obviously optimal $b_T$ should be 0. Then we can combine two parts together. Notice $a_T=1-\sum\limits_{i=1}^{T-1}a_i$. Which is to say, above problem is equivalent to:
\[
\max\limits_{b} \sum\limits_{i=1}^{T-1} a_i \{r^{i}  [M+\frac{r-1}{r} b_i]-Q\}
\]
where $Q=Mr^T$. For $\forall p\le T-1$, we have:
\[\sum\limits_{i=1}^{T-1}  a_i\{r^{i} [M+\frac{r-1}{r} b_i]-Q\}=\sum\limits_{i=1}^{p-1} a_i\{r^{i} [M+\frac{r-1}{r} b_i]-Q\}+\prod\limits_{j=1}^{p-1}(1-S_j)[S_p \{r^{p} [M+\frac{r-1}{r} b_p]-Q\}+(1-S_p)L_p],\] where \[L_p=\sum\limits_{i=p+1}^{T-1}  \{r^{i} [M+\frac{r-1}{r} b_i]-Q\} S_i \prod\limits_{k=p+1}^{i-1} (1-S_j)\]
(In the case $N_1>N_2$, let $\sum\limits_{N_1}^{N_2} = 0 $ and $\prod\limits_{N_1}^{N_2} = 1 $.)
F.O.C requires the following equation must hold for the optimal bonus structure ($L_p$ is irrelevant with $b_p$):
\[
h(b_p) [r^p (M+\frac{r-1}{r} b_p)-Q]+H(b_p)r^p \frac{r-1}{r}-h(b_p)L_p=0\] 
which can be simplified as:
\[
\frac{r-1}{r}\beta(b_p)+M=\frac{L_p+Q}{r^p}
\]
We can check the second order condition, the left hand side should be 
\[[r^p(M+\frac{r-1}{r}b_p)-L_p-Q]h'(b_p)+2h(b_p)r^p \frac{r-1}{r}\]
and if it's minimum solution we want it to be positive. Combine with the FOC we know it's equal to
\[-[H(b_p)r^p\frac{r-1}{r}]h'(b_p)+2h^2(b_p)r^p \frac{r-1}{r}\]
By Assumption \ref{assumption:monotone_beta} we know the fact that $\beta(x)$ is increasing implies $2h^2(x)-H(x)h'(x)> 0$ for sure. Hence SOC is satisfied.
Moreover, from the definition of $L_p$, we know that for $p\le T-2$:
\[
\begin{split}
L_p=\sum\limits_{i=p+1}^{T-1}  \{r^{i} [M+\frac{r-1}{r} b_i]-Q\} S_i \prod\limits_{k=p+1}^{i-1} (1-S_j) \\
=(1-S_{p+1})\sum\limits_{i=p+2}^{T-1}   \{r^{i} [M+\frac{r-1}{r} b_i]-Q\} \prod\limits_{k=p+2}^{i-1} (1-S_j)+\{r^{p+1}[M+\frac{r-1}{r}b_{p+1}]-Q\} S_{p+1}\\
=(1-S_{p+1})L_{p+1}+\{r^{p+1}[M+\frac{r-1}{r}b_{p+1}]-Q\} S_{p+1}\\
\end{split}
\]
which is to say
\[L_p+Q=(1-S_{p+1})(L_{p+1}+Q)+r^{p+1}[M+\frac{r-1}{r}b_{p+1}]S_{p+1}\]
Then the F.O.C implies
\[\frac{1}{r}[\frac{r-1}{r}\beta(b_p)+M]=(1-S_{p+1})[\frac{r-1}{r}\beta(b_{p+1})+M]+[\frac{r-1}{r}b_{p+1}+M]S_{p+1}\]
which is equivalent to
\begin{equation}
    \beta(b_p)=r\psi(b_{p+1})
    \label{equation_FOC_FC}
\end{equation}
And for $p=T-1$ we can still expand $a_{T-1}$. We are trying to maximize $a_{T-1}[r^{T-1}(M+\frac{r-1}{r}b_{T-1})-Mr^T]$, which is equivalent to 
\[\max_{b_{T-1}} H(b_{T-1})[(1-r)M+\frac{r-1}{r}b_{T-1}]\]
hence the FOC for $b_{T-1}$ is like
\[b_{T-1}+\frac{H(b_{T-1})}{h(b_{T-1})}=rM\]
since $b_T=0,\text{ and }\psi(0)=M$, we can rewrite it as $\beta(b_{T-1})=r\psi(b_T)$. Hence equation (\ref{equation_FOC_FC}) holds for $\forall p\le T-1$
And SOC holds too. Combining the above two equations we can finish the proof of this recursive structure for $\forall p\le T-1$. We need the following facts to guarantee the sequence $\{b_t\}$ is monotone:

\begin{fact}
    $\beta(x)-\frac{H^2(x)}{h(x)}$ is monotone increasing
     \label{fact_monotone}
\end{fact}
\begin{proof}
   Its first order derivation is $\frac{[1-H(x)][2h^2(x)-H(x)h'(x)]}{h^2(x)}>0$ ( from Assumption \ref{assumption:monotone_beta}) for any $x\in [0,\bar c)$.
\end{proof}

\begin{fact}
      $(\frac{1}{r}-1)\beta(x)+\frac{H^2(x)}{h(x)}$ is monotone increasing
      \label{fact_monotone_complex}
\end{fact}
\begin{proof}
   Its first order derivation is $[\frac{1}{r}-1+H(x)]\frac{2h^2(x)-H(x)h'(x)}{h^2(x)}>0$ ( from Assumption \ref{assumption:monotone_beta}, and $r<1$) for any $x\in [0,\bar c)$.
\end{proof}

\begin{fact}
	$b_{p+1}<b_p<b^*$ given $0<b_{p+1}<b^*$.
 \label{factgammaincrease}
\end{fact}
\begin{proof}
	$\beta(b_p)-\beta(b_{p+1})=r[M-\frac{H^2(b_{p+1})}{h(b_{p+1})}+\beta(b_{p+1})]-\beta(b_{p+1})>r[M-\frac{H^2(b^*)}{h(b^*)}+\beta(b^*)]-\beta(b^*)=0$ hence $b_p>b_{p+1}$. \\
	On the other hand $\frac{\beta(b_p)}{r}=M-\frac{H^2(b_{p+1})}{h(b_{p+1})}+\beta(b_{p+1})<M-\frac{H^2(b^*)}{h(b^*)}+\beta(b^*)=\frac{\beta(b^*)}{r}$ hence $b_p<b^*$
\end{proof}
Then we finish the proof of Lemma \ref{FC_lemma_finite}.
\end{proof}
\subsection{Proof of Proposition \ref{FC_proposition_finite}}
\label{section_proof_proposition_4_3}
\begin{proof}
Given Lemma \ref{FC_lemma_finite}, we only need to take care of the existence of $b_p$ and whether it's valid (i.e. lies in interval $[0,b^*]$). The following fact is enough to finish our proof for the finite case.
\begin{fact}
	$b_{T-1}<b^*$ given $b_T=0$.
\end{fact}
\begin{proof}
	  Fact \ref{fact_monotone_complex} guarantees $\beta(x)-\frac{H^2(x)}{h(x)}$ is monotone increasing. Then we know:
	$\frac{\beta(b_{T-1})}{r}=M+\beta(0)-\frac{H^2(0)}{h(0)}=M=\frac{H^2(b^*)}{h(b^*)}+(\frac{1}{r}-1) \beta(b^*)<\beta(b^*)+(\frac{1}{r}-1) \beta(b^*)=\frac{\beta(b^*)}{r}$ , hence $b_{T-1}=\Gamma(0)<b^*$
\end{proof}

Hence starting from $b_T=0$ we get the $b_t$ sequence and it's monotonically increasing with respect to $t$, i.e. $b^*>b_1>b_2>\cdots>b_{T-1}>b_T=0$. So if $T=1$ we have $b_T=0$ hence it's actually a Non-Bonus Strategy. Otherwise we have $b_1>0$ hence it's a Full Coverage Strategy. 
Up to now we have provided the proof for finite part of Proposition \ref{FC_proposition_finite}.

When $T=\infty$, actually Lemma \ref{FC_lemma_finite} still works hence we know the optimal $b^*$ is the solution for equation $\frac{\beta(x)}{r}=\psi(x)$. However a more safe way is to use the value function like
\[V=\max_x H(x)[\mathbb ER_1-x+\mathbb E\max\{R_1,R_2\}\frac{r}{1-r}]+(1-H(x))[\mathbb ER_1+rV]\]
hence F.O.C. is
\[\beta(x)=\mathbb E\max\{R_1,R_2\}\frac{r}{1-r}-rV\]
Using F.O.C to replace $V$ in goal function we get
\[[1-r+rH(x)][\mathbb E\max\{R_1,R_2\}\frac{r}{1-r}-\beta(x)]=r\mathbb ER_1+rH(x)[\mathbb E\max\{R_1,R_2\}\frac{r}{1-r}-x]\]
hence for the solution $b^*=x$ we have:
\[\beta(x)=r\psi(x)\]
and 
\[V=\mathbb E\max\{R_1,R_2\}\frac{1}{1-r}-\psi(b^*)\]
As before we can guarantee that $b^*$ lies in the interval $(0,\bar c)$ hence when $T=\infty$, the optimal Full Coverage (including Non Bonus) strategy is to set $b_i\equiv b^*$.
\end{proof}

\newpage
\subsection{Proof of Partial Coverage: Proposition \ref{PC_proposition_finite}}
\label{section_proof_proposition_4_4}
\subsubsection{Proof of Proposition \ref{PC_proposition_finite}}
\begin{proof}
If the platform uses partial coverage strategy and the reporting happens at period $t_0\le T$, then the profit is:
\[R_2(1+r+..+r^{t_0-2})+\mathbb E R_1r^{t_0-1}+\mathbb E \max\{R_1,R_2\}(r^{t_0}+..+r^{T-1})-\mathbb E cost\]
with the same notation $a_i \forall 1\le i \le T$ defined in the proof of Lemma \ref{FC_lemma_finite}, we have profit=

\[\begin{aligned}
	\sum\limits_{i=1}^T Pr(t_0=i)[R_2\frac{1-r^{t_0}}{1-r}+(\mathbb ER_1-R_2) r^{t_0-1}+\mathbb E\max\{R_1,R_2\}\frac{r^{t_0}-r^T}{1-r}-b_{t_0}r^{t_0-1} ]\\+Pr(\text{no reports}) R_2\frac{1-r^T}{1-r}\\
	=\sum\limits_{i=1}^{T-1} Pr(t_0=i)[R_2\frac{1-r^{t_0}}{1-r}+(\mathbb ER_1-R_2) r^{t_0-1}+\mathbb E\max\{R_1,R_2\}\frac{r^{t_0}-r^T}{1-r}-b_{t_0}r^{t_0-1} ]\\+a_T R_2\frac{1-r^T}{1-r}+Pr (t_0=T )( (\mathbb ER_1-R_2)r^{T-1}-b_T r^{T-1})\\
	=\sum\limits_{i=1}^{T-1} a_i [\frac{R_2-\mathbb E\max\{R_1,R_2\} r^T}{1-r}+\frac{(\frac{(\mathbb ER_1-R_2)(1-r)}{r}+\mathbb E\max\{R_1,R_2\}-R_2)r^i}{1-r}-b_ir^{i-1} ]\\+a_T R_2\frac{1-r^T}{1-r}+Pr (t_0=T )( (\mathbb ER_1-R_2)r^{T-1}-b_T r^{T-1})\\
	=(1-a_T)\frac{R_2-\mathbb E\max \{R_1,R_2\}r^T}{1-r}+\sum\limits_{i=1}^{T-1} a_i r^i\frac{N-b_i(1-r)/r}{1-r}+\\+a_T R_2\frac{1-r^T}{1-r}+Pr (t_0=T )( (\mathbb ER_1-R_2)r^{T-1}-b_T r^{T-1})\\
	=\sum\limits_{i=1}^{T-1} a_i r^i\frac{N-b_i(1-r)/r}{1-r}+Pr (t_0=T )( (\mathbb ER_1-R_2)r^{T-1}-b_T r^{T-1})+\\a_T\frac{(\mathbb E\max\{R_1,R_2\}-R_2) r^T}{1-r}+constant
\end{aligned}\]

Where we denote $N=M+\frac{\mathbb E R_1-R_2}{r}$. Notice $a_T=1-\sum\limits_{i=1}^{T-1}a_i$, the above problem is equivalent to:
\[\max\limits_{b_T} H(b_T)(\mathbb E R_1-R_2-b_T)\]
and
\[
\max\limits_{b} \sum\limits_{i=1}^{T-1}   a_i \{r^{i}[N+\frac{r-1}{r} b_i]-W\}\]
where $W=(\mathbb E\max\{R_1,R_2\}-R_2) r^T$.

We first solve the optimal $b_T$. We should notice that unlike $M$ is always positive, $N$ may be negative. Unlike the case in full coverage, it's possible that $b_T$ is positive or negative.  The optimal $b_T$ satisfies F.O.C:
\[\beta(b_T)=ER_1-R_2\]
And S.O.C. satisfies according to assumption \ref{assumption:monotone_beta}
This result shows that when $R_2$ is very large, the optimal $b_T$ may be negative, and the consumers would choose arm 2 to get utility 0 instead of a negative utility  $-\epsilon$ by purchasing arm1 since he will never report to get a negative bonus and pay a reporting cost. 

As for the $b_t,\forall t\le T-1$, we claim the recursive relation for interior solution using such a lemma:
\begin{lemma}
	Suppose that there exists $1\leq p<T$ such that the corresponding optimal bonus scheme satisfies $0<b_p<\bar c$. Then we have the following recursive relationship:
	\begin{equation}
		\frac{\beta(b_p)}{r}=\psi_N(b_{p+1}),\label{recurrence_N}
	\end{equation}
	where $N=M+\frac{\mathbb E R_1-R_2}{r}$ and $M=\mathbb E\max\{R_1,R_2\}-\mathbb ER_1$ and $\psi_N(\cdot)$ as denoted ahead.
 \label{PC_lemma_finite} 
\end{lemma}
\begin{proof}
Like the proof of Lemma \ref{FC_lemma_finite} before, for $\forall p\le T-1$, we have:
\[\sum\limits_{i=1}^{T-1}  a_i\{r^{i} [N+\frac{r-1}{r} b_i]-W\}=\sum\limits_{i=1}^{p-1} a_i\{r^{i} [N+\frac{r-1}{r} b_i]-W\}+\prod\limits_{j=1}^{p-1}(1-S_j)[S_p \{r^{p} [N+\frac{r-1}{r} b_i]-W\}+(1-S_p)L_p] \] where \[L_p=\sum\limits_{i=p+1}^{T-1}  \{r^{i} [N+\frac{r-1}{r} b_i]-W\} S_i \prod\limits_{k=p+1}^{i-1} (1-S_j)\]
Notice it's only valid for $p\le T-2$.
F.O.C requires the following equation must hold for the optimal bonus structure ($L_p$ is irrelevant with $b_p$):
\[
h(b_p) [r^p (N+\frac{r-1}{r} b_p)-W]+H(b_p)r^p \frac{r-1}{r}-h(b_p)L_p=0\] 
which can be simplified as:
\[
\frac{r-1}{r}\beta(b_p)+N=\frac{L_p+W}{r^p}
\]
We can check the second order condition, the left hand side should be 
\[[r^p(N+\frac{r-1}{r}b_p)-L_p-W]h'(b_p)+2h(b_p)r^p \frac{r-1}{r}\]
and if it's minimum solution we want it to be positive. Combine with the FOC we know it's equal to
\[[H(b_p)r^p\frac{r-1}{r}]h'(b_p)+2h^2(b_p)r^p \frac{r-1}{r}\]
By Assumption \ref{assumption:monotone_beta} we know the fact that $\beta(x)$ is increasing implies $2h^2(x)-H(x)h'(x)> 0$ for sure. Hence SOC is satisfied.

Moreover, from the definition of $L_p$, we know that for $p\le T-2$:
\[
\begin{split}
L_p=\sum\limits_{i=p+1}^{T-1}  \{r^{i} [N+\frac{r-1}{r} b_i]-W\} S_i \prod\limits_{k=p+1}^{i-1} (1-S_j) \\
=(1-S_{p+1})\sum\limits_{i=p+2}^{T-1}   \{r^{i} [N+\frac{r-1}{r} b_i]-W\} \prod\limits_{k=p+2}^{i-1} (1-S_j)+\{r^{p+1}[N+\frac{r-1}{r}b_{p+1}]-W\} S_{p+1}\\
=(1-S_{p+1})L_{p+1}+\{r^{p+1}[N+\frac{r-1}{r}b_{p+1}]-W\} S_{p+1}\\
\end{split}
\]
which is to say
\[L_p+W=(1-S_{p+1})(L_{p+1}+W)+r^{p+1}[N+\frac{r-1}{r}b_{p+1}]S_{p+1}\]
hence 
\[\frac{1}{r}[\frac{r-1}{r}\beta(b_p)+N]=(1-S_{p+1})[\frac{r-1}{r}\beta(b_{p+1})+N]+[\frac{r-1}{r}b_{p+1}+N]S_{p+1}\]
which is equivalent to
\[\beta(b_p)=r\psi_N(b_{p+1})\]
\end{proof}

However, unlike the case in Full Coverage, where we have the recursive structure and guarantee the interior solutions are valid hence the optimal structure is clear. In Partial Coverage case, having Lemma \ref{PC_lemma_finite} is not enough to get the final PC (containing SA) solutions. The reason is there may be negative interior bonus. But given $b_{p+1}<0$, which we should treat as $b_{p+1}=0$, $b_p$ will solve the F.O.C. for  $b_{p+1}=0$ hence breaks the recursive rule.

%If $b_T<0$, from equation (\ref{recurrence_N}) we know the every point of the interior solution sequence is negative. Hence in this case, the bonus structure is equivalent to set $(0,0,..0)$.
Then we discuss the optimal solution given above interior recursive structure. Unlike Full Coverage case, we can't guarantee $b_t\ge 0$ here. Hence, for simplicity, we use sequence $\{d_t\}$ for the interior solution, allowing distribution functions have similar functional form outside the support, and $\{b_t\}$ for the final results, taking validity (i.e. valid $b$ should be positive) into consideration. 
we should notice the following facts:
\begin{fact}
~\\
If $N>0$, then equation  \[(\frac{1}{r}-1)\beta(x)+\frac{H^2(x)}{h(x)}=N\] has solution
$b_N^*>0$ 

If $\mathbb ER_1-R_2>0$, the equation 
 \[\beta(x)=\mathbb ER_1-R_2\]
have solution  $b_T>0$. Otherwise denote $b_T=0$.
    \label{PC_fact_signal}
\end{fact}

\begin{proof}

    We have shown in Fact \ref{fact_monotone_complex} that the left hand side is monotonically increasing with respect to $x$ and gets 0 when $x=0$. So given a positive $N$, we get $d_N^*>0$. Otherwise we can not find a valid $d_N^*>0$ (However, in numerical solutions we can still solve a negative one if we let $\beta(x)=2x, \forall x$).

    Similarly, $b_T$ solves
    \[\beta(x)=\mathbb ER_1-R_2\] and the same logic works for $\beta(\cdot)$.
\end{proof}
\begin{fact}
    ~\\
    There are three contingencies for the sequence $\{b_t\}$.  An numerical illustration for the second and the third case are shown in  Figure \ref{bTneg} and Figure \ref{bTnegNneg}, if we simply let $H(x)= x ( \text{ instead of }x \mathbb I[0,1])$ and $h(x)=1 (\text{ instead of }1\mathbb I[0,1])$, i.e. ignore the fact that $h(x)$ and $H(x)$ is not defined outside the interval [0,1].
    \begin{itemize}
        \item If $N>0$ and $d_T>0$, we have $d_N^*>d_1>d_2>d_3>...>d_{T-1}>d_T>0$. Hence in this case $b_t=d_t$. 
        \item If $N>0$ and $d_T<0$, we have $d_N^*>d_1>d_2>d_3>...>d_{T-1}>0>d_T$. Hence in this case $b_t=d_t$ for $t\le T-1$ and $b_T=0$.
        \item If $N<0$, we have $0>d_N^*>d_1>d_2>d_3>...>d_{T-1}>d_T$. Hence in this case $0=b_N^*=b_1=b_2=b_3=...=b_{T-1}=b_T$.
    \end{itemize}
    \label{PC_fact_sequence}
\end{fact}
\begin{proof}
	From the definition of $b_N^*$ we know $(\frac{1}{r}-1)\beta(b_N^*)+\frac{H^2(b_N^*)}{h(b_N^*)}=N=M+\frac{\mathbb ER_1-R_2}{r}$, and $(\frac{1}{r}-1)\beta(b_T)+\frac{H^2(b_T)}{h(b_T)}=(\mathbb ER_1-R_2)(\frac{1}{r}-1)+\frac{H^2(b_T)}{h(b_T)}=\frac{H^2(b_T)}{h(b_T)}+R_2-\mathbb ER_1+\frac{\mathbb ER_1-R_2}{r}$. 
 
    In the first case, if $b_T>0$, we have $\beta(b_T)-\frac{H^2(b_T)}{h(b_T)}>\beta(0)-\frac{H^2(0)}{h(0)}=0$, hence $\frac{H^2(b_T)}{h(b_T)}+R_2-\mathbb ER_1+\frac{\mathbb ER_1-R_2}{r}<\beta\left(b_T\right)+R_2-\mathbb ER_1+\frac{\mathbb ER_1-R_2}{r}=0+\frac{\mathbb ER_1-R_2}{r}<M+\frac{\mathbb ER_1-R_2}{r}=N$, hence $b_T<b_N^*$. Then with the same logic above, this inequality can be iterated, hence we finish the proof of the first part here.
	
	When $b_T<0$, the direction of inequality changes. Actually above function is not defined when $b_T<0$. However, with our basic definition, $\psi_N(x)=\beta(x)-\frac{H^2(x)}{h(x)}+N$, and when $x<0$ it degenerates into simply $N$. Hence in the first step we have $\beta(b_{T-1})=rN$, which will lead to a positive $b_{T-1}$. In this case, we have $(\frac{1}{r}-1)\beta(b_N^*)+\frac{H^2(b_N^*)}{h(b_N^*)}=N=M+\frac{\mathbb ER_1-R_2}{r}$, and $(\frac{1}{r}-1)\beta(b_{T-1})+\frac{H^2(b_{T-1})}{h(b_{T-1})}=rN(\frac{1}{r}-1)+\frac{H^2(b_{T-1})}{h(b_{T-1})}=\frac{H^2(b_{T-1})}{h(b_{T-1})}+rN(\frac{1}{r}-1)$. Since $b_{T-1}>0$, we have $\beta(b_{T-1})-\frac{H^2(b_{T-1})}{h(b_{T-1})}>\beta(0)-\frac{H^2(0)}{h(0)}=0$, hence $\frac{H^2(b_{T-1})}{h(b_{T-1})}+rN(\frac{1}{r}-1)<\frac{H(b_{T-1})}{h(b_{T-1})}+b_{T-1}+rN(\frac{1}{r}-1)=0+N$, hence $b_{T-1}<b_N^*$. And with the same logic in the first part, we have $b_N^*>b_1>b_2>\cdots>b_{T-1}>0$.
	
	Moreover, we should notice that when $x<0$, $\beta(x)$ degenerates to $\beta(x)=x$ and $\psi_N(x)$ degenerates to $\psi_N(x)=x+N$. Hence given  $N<0$, $\beta(b_{T-1})=\psi_N(b_T)=b_T+N<0$ so we should set $b_{T-1}=0$. The same logic guarantees $b_i=0,\forall i$. 
\end{proof}

\begin{figure}[H]
	\begin{minipage}[t]{0.5\linewidth}
		\centering
		\includegraphics[scale=0.5]{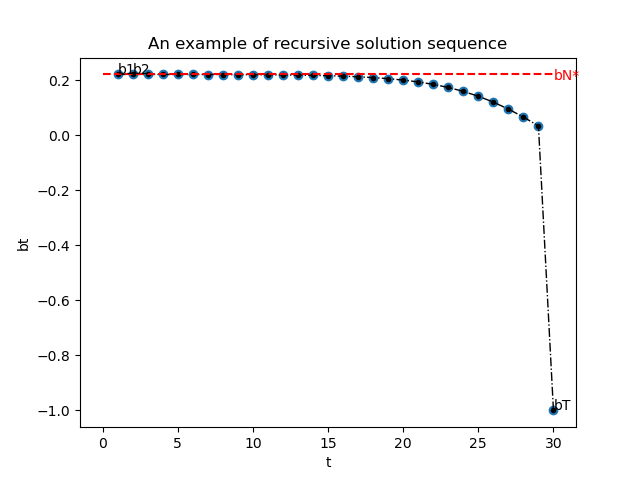}
		\caption{$b_T<0$ and $N>0$}
		\label{bTneg}
	\end{minipage}%
	\begin{minipage}[t]{0.5\linewidth}
		\centering
		\includegraphics[scale=0.5]{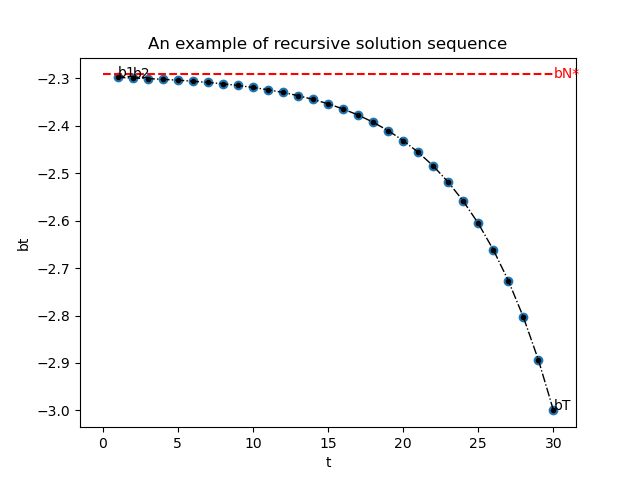}
		\caption{$b_T<0$ and $N<0$}
		\label{bTnegNneg}
	\end{minipage}
\end{figure}

Last but not least, we should point out that the second part in Assumption  \ref{assumption_exist_bstar} actually rules IR out in PC cases, since the same logic works in the proof of Lemma \ref{FC_lemma_finite}.
Lemma \ref{PC_lemma_finite}, combined with Fact \ref{PC_fact_signal} and \ref{PC_fact_sequence} finishes proof of finite part in Proposition \ref{PC_proposition_finite}.   

When $T\to \infty$, we again use the value function way.
\[V=\max_x H(x)[\mathbb ER_1-x+\mathbb E\max\{R_1,R_2\}\frac{r}{1-r}]+(1-H(x))[R_2+rV]\]
hence F.O.C. is
\[\beta(x)=\mathbb E\max\{R_1,R_2\}\frac{r}{1-r}-rV+\mathbb ER_1-R_2\]
Using F.O.C to replace $V$ in goal function we get
\[r\mathbb E\max\{R_1,R_2\}+(\mathbb ER_1-R_2-\beta(x))(1-r)-r\frac{H^2(x)}{h(x)}=rR_2\]
hence
\[\beta(b_N^*)=r\psi_N(b_N^*)\]
and
\[V=\mathbb E\max\{R_1,R_2\}\frac{1}{1-r}-\psi_N(b_N^*)-\frac{\mathbb ER_1-R_2}{r}\]
Then from Fact \ref{PC_fact_signal} we know exists $b_N^*>0\Leftrightarrow N>0$, and Assumption \ref{assumption_exist_bstar} guarantees that $b_N^*<\bar c$. Hence we should use Partial Coverage when $N>0$ and otherwise Safe Arm.
\end{proof}
\newpage

\subsection{Proof of Lemma \ref{optimal_lemma}(total utility)}
\label{section_proof_total_utility}
\begin{proof}
If $T=\infty$, we have got the expression of its utility in the proof of proposition \ref{FC_proposition_finite} and proposition \ref{PC_proposition_finite}. 

When $T$ is finite, we denote $\eta_p$ to be the total utility of bonus structure \[(0,0,...0,\Gamma^{(p)}(b_T),\Gamma^{(p-1)}(b_T),..\Gamma^{(1)}(b_T),b_T).\] Hence obviously we have the following equation by denoting $x=\Gamma^{(p)}(b_T)$:
\[\begin{split}
\eta_p=\mathbb E R_1(1+r+..r^{T-p-1})-H(x)xr^{T-p-1}+H(x)\mathbb E\max\{R_1,R_2\}(r^{T-p}+r^{T-p+1}+..r^{T-1})\\+[1-H(x)][\eta_{p-1}-\mathbb E R_1(1+r+..r^{T-p-1})]\\
=H(x)\mathbb ER_1\frac{r^{T-p}-1}{r-1}-H(x)xr^{T-p-1}+H(x)\mathbb E\max\{R_1,R_2\}r^{T-p}\frac{r^{p}-1}{r-1}+(1-H(x))\eta_{p-1}
\end{split}\]

We have known $x=\Gamma^{(p)}(b_T)$ maximizes $\eta_p$ given $\eta_{p-1}$ fixed. Hence F.O.C. must hold for $x=\Gamma^{(p)}(b_T)$, thus we can get the expression of $\eta_{p-1}$ (we just use the it as a necessary condition here so we don't need to check S.O.C., which has been satisfied before): 
\[\eta_{p-1}=\mathbb E\max\{R_1,R_2\}\frac{r^T-r^{T-p}}{r-1}+\mathbb E R_1\frac{r^{T-p}-1}{r-1}-r^{T-p-1} \beta(x)\]
hence
\[\eta_{p-1}=\mathbb E\max\{R_1,R_2\}\frac{r^T-r^{T-p}}{r-1}+\mathbb E R_1\frac{r^{T-p}-1}{r-1}-r^{T-p} \psi(\Gamma^{(p-1)}(0))\]

Hence $\eta_{T-1}=\mathbb E\max\{R_1,R_2\}\frac{r^T-1}{r-1}-\psi(b_1)$.
Similarly, if the platform uses Partial Coverage Strategy, we have 
\begin{equation}
\begin{split}
\eta_p=H(x)[R_2(1+r+..r^{T-p-2})+\mathbb ER_1r^{T-p-1}-xr^{T-p-1}+\mathbb E\max\{R_1,R_2\}(r^{T-p}+r^{T-p+1}+..r^{T-1})]\\+[1-H(x)]\eta_{p-1}\\
=H(x)[R_2\frac{r^{T-p-1}-1}{r-1}+R_1r^{T-p-1}-xr^{T-p-1}+\mathbb E\max\frac{r^T-r^{T-p}}{r-1}]+[1-H(x)]\eta_{p-1} \label{rec_par_cov}
\end{split}
\end{equation} 

From above analysis we know the platform chooses the optimal $x$ to maximize $\eta_p$ given $\eta_{p-1}$, hence the F.O.C must hold at $x$ :
\begin{equation*}
\eta_{p-1}=-\beta(x)r^{T-p-1}+R_2\frac{r^{T-p-1}-1}{r-1}+\mathbb ER_1r^{T-p-1}+\mathbb E\max\{R_1,R_2\}\frac{r^T-r^{T-p}}{r-1}
\end{equation*}

This equation should hold for $\forall 1\le p\le T-1$, hence let $p=T-1$,  $\eta_{T-2}=-\beta(x)+\mathbb ER_1+\mathbb E\max\{R_1,R_2\}\frac{r^T-r}{r-1}$ where $x=b_{N_1}$. Plug this result in to the recursive equation (\ref{rec_par_cov}) at $p=T-1$, we can get the final $\eta_{T-1}$:
\begin{equation}
\eta_{T-1}=\mathbb E\max\{R_1,R_2\}\frac{r^T-1}{r-1}-\psi(b_{N_1})
\end{equation}
where $b_{N_1}=\Gamma_N^{(T-1)}(b_T)$. Notice it's $\psi(b_{N_1})$ instead of $\psi_N(b_{N_1})$. To ensure, consider the case when $T=1$. F.O.C. is $\beta(b_T)=ER_1-R_2$, and the value function is
\[\begin{aligned}
    H(b_T)(\mathbb ER_1-b_T)+(1-H(b_T))R_2=H(b_T)[\beta(b_T)-b_T]+R_2\\=H(b_T)\frac{H(b_T)}{h(b_T)}+R_2-\mathbb E R_1+\mathbb E R_1\\
    =H(b_T)\frac{H(b_T)}{h(b_T)}-\beta(b_T)+\mathbb E R_1+\mathbb E\max\{R_1,R_2\}-\mathbb E\max\{R_1,R_2\}\\
    =\mathbb E\max\{R_1,R_2\}-\psi(b_T)
\end{aligned}\]

Here is an example to show that this result is robust when sequence $\{b_t\}$ contains negative items (Actually the negative item also fits equation (\ref{rec_par_cov}), when $b_p<0$, $\eta_p=\eta_{p+1}$). For example, only $b_1>0$ and $b_2,b_3,..b_T=ER_1-R_2<0$. The recursive relation for $t\ge 2$ is $\frac{\beta(b_p)}{r}=\psi_N(b_{p+1}) \Rightarrow \frac{b_p}{r}=N+b_{p+1}$. Hence $b_t+\frac{rN}{r-1}=r^{T-t}(b_T+\frac{rN}{r-1})$. The above result shows $\eta_{T-2}=-\beta(\Gamma^{(T-1)}(b_T))+R_1+Emax\{R_1,R_2\}\frac{r^T-r}{r-1}$. Combine these two results together we can get $\eta_{T-2}=\frac{r^T-1}{r-1}R_2$, which fits the direct calculation given structure $b_2,b_3,..b_T=ER_1-R_2<0$.
\end{proof}
\subsection{Numeric Examples in Section \ref{Section_Discrete_Analysis}}
\subsubsection{Details for Figure \ref{3totalUR2}}
We consider $R_1\sim U[0,4],c\sim U[0,1],T=2$. Hence $M=Emax\{R_1,R_2\}-ER_1=\frac{R_2^2}{8}$. In RFC, given $b_2=0$, we know $\beta(b_1)=2b_1=r\psi_M(b_2)=rM$ so $b_1=\frac{rM}{2}=\frac{rR_2^2}{16}$. The root of $b_1=\bar c=1$ is $\frac{4}{\sqrt r}$, which is just the $\bar R_2$. In this case $\bar R_2>\bar c$ hence IRM should not be optimal, but we can make it real by choosing a large $T$.  In RPC, if $ER_1-R_2>0,b_2>0$,  $\beta(b_2)=2b_2=ER_1-R_2$, hence $\beta(b_{1N})=2b_1=\psi_N(b_2)$ which will lead to $b_{1N}=\frac{r}{2}[ER_1-R_2+N-\frac{(ER_1-R_2)^2}{4}]=\frac{r}{2}+1-\frac{R_2}{2}-\frac{rR_2^2}{16}$. The root of $b_{1N}=\bar c=1$ is our $\underline R_2$. Hence $b_1-b_{1N}=(R_2-2)(\frac{r}{8}R_2+\frac{2+r}{4})$. We predict before that $\hat R_2=ER_1$ and we can see it's true here.\\

$N=\frac{R_2^2}{8}-\frac{2-R_2}{r}$ hence the root of which is $\frac{4(1 \pm \sqrt{1-r})}{r}$. The smaller one, $\frac{4(1 - \sqrt{1-r})}{r}<4$ is $\tilde{R}_2$ as we analyzed before.

\subsubsection{Details for Figure \ref{rho_affects_bonus} }
\label{proof_rho}

To be more specific, if $x<3$ then $\rho x+(1-\rho)y<3\rho+3(1-\rho)=3$. Otherwise for any $x\in (3,4)$, we have $\rho x+(1-\rho)y>3$ requires $y>\frac{3-\rho x}{1-\rho}$. Then there are two cases. If $\frac{3-\rho x}{1-\rho}>1 \forall x\in[3,4]$ (i.e. $\rho<\frac{2}{3}$), then we know 
\[8 \mathbb E\max\{R_1,R_2\} = \int_0^3\int_1^3 3  dydx + \int_3^4 \int_1^{\frac{3-\rho x}{1-\rho}} 3 dy dx+\int_3^4 \int_{\frac{3-\rho x}{1-\rho}}^3 \rho x+(1-\rho)y dy dx\]
which is equal to 
\[18+\frac{12-15\rho}{2(1-\rho)}+\frac{\rho(\rho+9)}{6(1-\rho)}\]
whose differential with respect to $\rho$ is equal to
\[\frac{(2-\rho)\rho}{6(1-\rho)^2}>0\]

In the other case, we have
\[\begin{aligned}
    8 \mathbb E\max\{R_1,R_2\} = \int_0^3\int_1^3 3  dydx + \int_3^{\frac{2+\rho}{\rho}} \int_1^{\frac{3-\rho x}{1-\rho}} 3 dy dx+\\ \int_3^{\frac{2+\rho}{\rho}} \int_{\frac{3-\rho x}{1-\rho}}^3 \rho x+(1-\rho)y dy dx+\int_{\frac{2+\rho}{\rho}}^4 \int_1^3 \rho x+(1-\rho)y dy dx
\end{aligned}\]
which is equal to 
\[\frac{58}{3}+\frac{13\rho}{3}+\frac{4}{3\rho}\]
Again, it's differential for $\rho$ is equal to 
\[\frac{13}{3}-\frac{4}{3\rho^2}>0\]

We should notice that these two expressions meet at $\rho=\frac{2}{3}$ smoothly.

\subsubsection{To Provide a Comparison with Figure \ref{wrong_fc_pc}}
\label{ER1sim0X}
We assume $R_1\sim U[0,X]$ with $X\ge R_2=2$. In this case we have
\[\mathbb E\max\{R_1,R_2\} =\int_0^2 2 \frac{1}{X} dx+\int_2^X x \frac{1}{X} dx=\frac{X^2+4}{2X}\]
Using the technical results discussed before we can get such a illustration in figure \ref{utility_X}. The following figure carries the same message as shown in figure \ref{u_R2_infty} (infinite case) or figure \ref{3totalUR2} (finite case), but in a opposite direction: there exists two cutoffs which stands for the optimal switching between PC and FC (when $R_2=\mathbb ER_1$, and between  PC and SA (when $N=0$). Again, $NB$ is never optimal. Figure \ref{utility_X} is only for comparison with figure \ref{fig:correct_fcl_pcl}.

We emphasize here that $NB$ is never optimal in perfect learning cases, and we will show that in imperfect learning cases, the region where NB is optimal will shrink when $\lambda\to \infty$ (i.e. when learning tends to be perfect). An illustration can be found in Figure \ref{fig:lambda} .

\begin{figure}[H]
    \centering
    \includegraphics[width=0.5\linewidth]{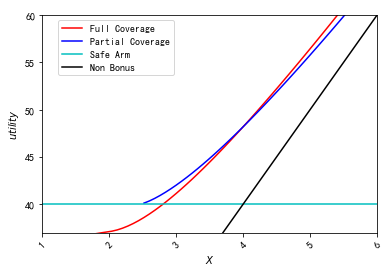}
    \caption{Profit-X When $T=\infty$}
    \label{utility_X}
\end{figure}

\newpage
\section{Appendix B: When Assumption\ref{assumption_exist_bstar} or \ref{assumption_barc_large} Fails}
\label{Section_IR}

\subsection{Discrete Immediate Revelation}
\label{Section_IR_discrete_statement}
In this subsection we consider the case when Assumption \ref{assumption_exist_bstar} is not satisfied, i.e. there is possibility that $d_1$ or $d_{N,1}$ is higher than $\bar c$ and hence the interior solution leads to the corner case. We should first notice that Assumption \ref{assumption_exist_bstar} requires a large enough $\bar c$ to rule out IR, and it's actually equivalent to $b^*<\bar c$. A modified version of Proposition \ref{FC_proposition_finite} and \ref{PC_proposition_finite}  should be as follows:

\begin{proposition}
	For $\forall T\ge 2$, construct the sequence $\{d_t\}$ as follows:
	\begin{enumerate}
		\item  if $T<\infty$, let $d_t=\Gamma^{(T-t)}(0)$ for $1\le t\le T$.
		\item  if $T=\infty$, let $d_t=b^*$ for $1\le t\le T$ ($b^*$ is the fixed point of function $\Gamma(\cdot)$ as declared in section 4.1).
	\end{enumerate}
	Then $d_1>0$ if $T>1$. Under our Assumption 3.1 and Assumption 3.2, the optimal full coverage strategy is to set:
	\begin{enumerate}
		\item  $(b_1,b_2,...b_T)=(d_1,d_2,...d_T)$, if $0<d_1<\bar c$  (i.e. using recursive structure).
		\item  $(b_1=\bar c,b_2=0,b_3=0,..b_T=0)$, if $d_1>\bar c$ (i.e., using immediate revelation) .
	\end{enumerate}
 \label{IR_fc}
\end{proposition}

\begin{proposition}
	For $\forall T\ge 2$, construct the sequence $\{d_t\}$ as follows:
	\begin{enumerate}
		\item  let $d_T$ to be the root of equation $\beta(d_T)=\mathbb ER_1-R_2$
		\item  if $T<\infty$, let $d_t=\Gamma_N^{(T-t)}(d_T)$ for $1\le t\le T$.
		\item  if $T=\infty$, let $d_t=b_N^*$ for $1\le t\le T$ ($b_N^*$ is the fixed point of function $\Gamma_N(\cdot)$ as declared in section 4.1).
	\end{enumerate}
	Under our Assumption \ref{Inada}, Assumption \ref{assumption:monotone_beta} and Assumption \ref{assumption_exist_bstar}, the optimal full coverage strategy is to set:
	\begin{enumerate}
		\item  $(b_{N1},b_{N2},...b_{NT})=(d_1,d_2,...d_T)$, if $0<d_1<\bar c$  (i.e. using recursive structure).
		\item  $(b_{N1}=\bar c,b_{N2}=0,b_{N3}=0,..b_{NT}=0)$, if $d_1>\bar c$ (i.e., using immediate revelation) .
		\item $(b_{N1}=0,b_{N2}=0,b_{N3}=0,..b_{NT}=0)$ if $d_1<0$ (i.e., setting non-bonus).
	\end{enumerate}
  \label{IR_pc}
\end{proposition}

Then back to the optimal strategy, by setting IR the platform can get profit $\pi_L=\mathbb E\max\{R_1,R_2\}\frac{1-r^T}{1-r}-M-\bar c  \text { if }  L=\text{Immediate Revelation}\\$
Combine this results with Lemma \ref{optimal_lemma}, we have a more complex comparative relationships like Proposition \ref{optimal_proposition}:

\begin{proposition}
	The comparison relationships between these four possible optimal strategies are as follows:
	\begin{center}
		$PC \prec FC \Leftrightarrow R_2<\bar {R}_2$ \\
		$FC \prec IR \Leftrightarrow R_2<\tilde R_2$\\
		$PC \prec IR \Leftrightarrow R_2>\tilde R'_2$\\
		$PC \prec SA \Leftrightarrow R_2>\hat{R}_2$ 
	\end{center} 
\label{proposition_IR}
\end{proposition}

An illustration of Proposition \ref{proposition_IR} can be found in Figure \ref{fig:FC_PC_SA_NB_IR_c01_T3} where we set $\bar c=0.1$ and $T=3$. We can still guarantee that $\bar R_2<\hat R_2$ but it's not sure where the $\tilde R_2$ or $\tilde R'_2$ lies. In other words, IR may be or may not be the optimal solution. Besides what we saw in figure 1 that FC tends to NB when $R_2$ is small, we can see FC tends to IR when $R_2$ is large, and PC tends to IR when $R_2$ is small.

Then we try to reveal some intuition by comparing IR vs FC.
Intuitively we know there are four incentives for the platform to use the highest bonus at the beginning (IR) : 
\begin{enumerate}
	\item when $T$ is large (many agents)
	\item  when $M=\mathbb E\max\{R_1,R_2\}-\mathbb ER_1$ is large (valuable information)
	\item when $\bar c$ is small (cheap process of information)
	\item when $r$ is large (future value matters)
\end{enumerate}

Above are four straightforward conditions which help $b_1>\bar c$ to hold, and our result fits these four insights well:

Firstly since $b_1=\Gamma^{(T-1)}(0)$, whether $b_1$ exceeds a fixed value $\bar c$ is actually a symbol of the size of $T$. We know the iteration of function $\Gamma$ is increasing from our Fact \ref{factgammaincrease}. Moreover, it's convergent from our proof of Lemma \ref{FC_lemma_finite}. Hence when $T$ is large enough, $b_1$ can get arbitrarily close to $b^*$, which will make it get over $\bar c$ as long as $b^*>\bar c$. The platform hence should use the upper bound bonus, $\bar c$, to get the information immediately. 

Points 2 and 3 are easy to understand. Holding everything else constant, a higher $M$ will lead to a higher $b_1$, hence makes $b_1<\bar c$ less important to hold hence provides more incentives to use ``Immediate revelation'' strategy. A smaller $\bar c$ directly makes $b_1<\bar c$ less important to hold (see figure \ref{FC_PC_SA_NB_IR_c04_T8} and \ref{FC_PC_SA_NB_IR_c1_T8} where $T=8,r=0.95,\mathbb ER_1=2$ in both cases, a lower $\bar c$ makes IR possible to be optimal).

\begin{figure}[h]
	\begin{minipage}[t]{0.45\linewidth}
		\centering
		\includegraphics[scale=0.5]{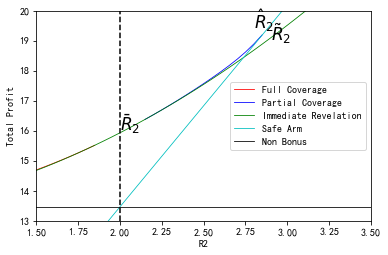}
		\caption{$\bar c=0.4, T=8$}
		\label{FC_PC_SA_NB_IR_c04_T8}
	\end{minipage}
	\begin{minipage}[t]{0.45\linewidth}
		\centering
		\includegraphics[scale=0.5]{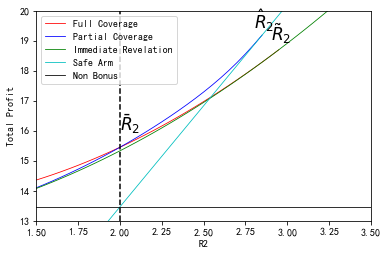}
		\caption{$\bar c=1, T=8$}
		\label{FC_PC_SA_NB_IR_c1_T8}
	\end{minipage}%
\end{figure}

\begin{figure}
    \centering
    \includegraphics[scale=0.7]{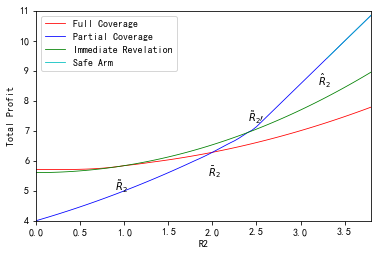}
    \caption{Profit-$R_2$ Under Different Strategies with IR}
    \label{fig:FC_PC_SA_NB_IR_c01_T3}
\end{figure}

\subsubsection{Proof of Proposition \ref{IR_fc} and \ref{IR_pc}}
\label{Section_IR_discrete_proof}

\begin{proof}

\begin{fact}
	For any $\{b_i\}$ and $x>0$, setting $b_p=x>0$ and $b_{p-1}=0$ is always (strictly) dominated by setting $b_p=0$, $b_{p-1}=x$ and remaining others.
 \label{neverzerobeforepositive}
\end{fact}
\begin{proof}
	$u(r_1,..r_p-1,x,0,r_{p+2,..})-u(r_1,..r_p-1,0,x,r_{p+2,..})=r^{p-1} \prod\limits_{j=1}^{p-1}(1-H(r_j))H(x)[Mr-x(1-r)]\ge r^{p-1} \prod\limits_{j=1}^{p-1}(1-H(r_j))H(x)[Mr-\bar c(1-r)]\ge 0$
\end{proof}

Given Fact \ref{neverzerobeforepositive}, we know it's impossible to set $b_{p-1}=0$ before any positive $b_{p}$. Hence we have to set $b_{p-1}=\bar{c}$ when corner solution is necessary. The next problem is given $b_p=\bar{c}$, what should $b_{p-1}$ be. Based on the fact that the recurrence relationship is monotone increasing we know the interior solution is even larger than $\bar c$ hence corner solution is again needed, combine with Fact \ref{neverzerobeforepositive} we know the only possible solution is to use $\bar c$. With the same logic we should set $b_{p-2}=...=b_1=\bar c$, then we can get our lemma , which is a key step in forming the optimal structure.
\begin{lemma}
	The bonus structures where $\exists p,s.t. b_p=\bar{c}$, is always dominated by setting $b_1=\bar{c}$.
 \label{IR_lemma}
\end{lemma}
Lemma \ref{IR_lemma} and Lemma \ref{FC_lemma_finite} are enough to prove our proposition  \ref{IR_fc}. With the same logic we can prove our proposition \ref{IR_pc}. 

\end{proof}

\subsection{Continuous Immediate Revelation}
\label{section_small_barc}
 
\setcounter{figure}{0} 
Assumption \ref{assumption_barc_large} is trying to simplify our analysis since in the text we want to focus on the Full Coverage and Partial Coverage. However, we can characterize the value function satisfied under Immediate Revelation. 
\[(r+\alpha \lambda )\Pi_{IR}(\alpha)=(\alpha z r\lambda -r\bar c)+(\alpha^2-\alpha)\lambda \Pi_{IR}'(\alpha)+\alpha \lambda^2 z \tag{IR-ODE}\]

Now we prove Assumption 5.1 is a sufficient but not necessary condition to ignore the existence of Immediate Revelation. 
\begin{proof}
    We consider the ``Immediate Revelation Only'' monopolist who can only switch from Immediate Revelation to Safe Arm. We assume the switching cutoff is $\alpha_{IR}$, then similar as stated in section 5.2, the monopolist face a smooth pasting problem where there should exist cutoff belief $\alpha_{IR}$ such that 
    \[\Pi_{IR}(\alpha_{IR})=\tilde V,\Pi_{IR}'(\alpha_{IR})=0\]
    combined with equation (IR-ODE) we get 
    \[\alpha_{IR}=\frac{r(\bar c+s)}{\lambda (g-s)+r g}\]

\end{proof}

Again, there should be a switching problem between Immediate Revelation and Full Coverage. We denote the switching point as $\underline \alpha_0$. Unlike before, we can not know for sure the optimal switching condition when using IR. We know $\alpha_{IR}>\alpha_{PC}$, but it's not sure whether $\alpha_{IR}>\alpha_{FC}$. Actually given $\min\{\alpha_{FC},\alpha_{IR}>\alpha_{PC}\}$, we know both IR curve and the FC curve will optimally switch into PC instead of SA. Hence even $\alpha_{IR}>\alpha_{FC}$, there is still possibility that $\alpha_{IR}^{PC}>\alpha_{FC}^{PC}$ (switching goal is denoted here). Obviously the smaller the $\bar c$, the higher probability that IR performs better than FC. 

Otherwise, we should let FC to smooth paste to PC, and let the IR to smooth paste to FC (or NB). If the cutoff happens before $\alpha_{FC}^*$, the smooth pasting condition can be written as
\[\Pi_{IR}(\underline \alpha_0)=V(\underline \alpha_0),\Pi_{IR}'(\underline \alpha_0)=V'(\underline \alpha_0)\]
which gives the boundary condition of $\Pi(\cdot)$ here. 

There is also probability that the cutoff happens after $\alpha_{FC}^*$. In this case there is no smooth pasting condition, which means IR curve will meet NB curve in the form of intersect rather than tangent, since if we let $\Pi_{IR}=\alpha z\lambda$ we get 
\[(\alpha^2-\alpha)(z\lambda^2-\lambda \Pi'(\alpha))=-r\bar c\]
Hence we must have $\Pi'(\alpha)<\lambda z$.

It's quite counter-intuitive to find there is a discontinuity on $C(\alpha)$ in Monopolist setting. Mathematically,two reasons result in the jump from $\bar c$ to 0. Firstly, in this monopolist setting when Assumption \ref{assumption_barc_large} is not satisfied, the monopolist will choose Immediate Revelation when $\alpha\to1$ where accordingly $C(\alpha)=\bar c$. But when the monopolist is optimal switching from IR to FC, it happens at the highest possible belief of FC interval. According to our insights get in the main text, though the monopolist faces a trade-off to set a high bonus in FC, $C(\alpha)$ in FC should still be monotonically decreasing for belief after the two trade-off effects are summed up. Hence at the jump point $C(\alpha)$ will jump from 1 to 0, given it's larger than $\alpha_{FC}^*$.

Moreover, for most times we can treat Assumption \ref{assumption_barc_large} as assuming a large enough $\bar c$. A simple and direct assumption is to assume $\bar c=\infty$, but it's hard to do the numerical illustration since it's hard to find a distribution function with infinite upper bound and 0 lower bound such that there exists explicit relationship between $\frac{H^2(\cdot)}{h(\cdot)}$ and $\beta(\cdot)$.
